# Supplementary material for: Polytope: Practical Memory Access Control for C++ Applications
Source: arXiv:2201.08461 source file (2022-01-24)
Supplement: Supplementary file 1 [file code_comparison_appendix.tex]

% !TEX main = main.tex
\begin{figure*}[h]
\centering
\begin{subfigure}[t]{0.45\linewidth}
\vskip 0pt
\centering    
\begin{lstlisting}[language=C,style=CStyle,linewidth=.9\linewidth]
//libmpk setup
#define GROUP_1 100

 int domain_based_isolation () {
 //libmpk initialization
 mpk_init(-1); 
 
 //manual explicit memory assignment from protected region
 char* addr = (char *) mpk_mmap(GROUP_1, NULL, 0x1000, PROT_READ | PROT_WRITE, MAP_ANONYMOUS | MAP_PRIVATE, -1, 0);

//manual entry, protected region start
mpk_begin(GROUP_1, PROT_READ | PROT_WRITE);

 // write data in GROUP_1
sprtintf(addr,"X");
//manual entry, protected region end
mpk_end(GROUP_1);
printf("%s\n", addr); // SEGMENTATION FAULT
\end{lstlisting}
~
\end{subfigure}
\begin{subfigure}[t]{0.45\linewidth}
\vskip 0pt
\centering    
\begin{lstlisting}[language=C,style=CStyle,linewidth=.9\linewidth]
//required Tesseract definitions
mpk_policy(VARIABLE)
mpk_partition(restricted)
...
int domain_based_isolation () {

mpk_local_control(no_access,restricted)
char* addr;
addr=malloc(0x1000);

mpk_actor_access(write,restricted)
sprtinf(addr,"X");

printf("%s\n", addr); // SEGMENTATION FAULT

\end{lstlisting}
\end{subfigure}

\begin{subfigure}[t]{0.45\linewidth}
\vskip 0pt
\centering    
\begin{lstlisting}[language=C,style=CStyle,linewidth=.9\linewidth]
//ERIM setup 
..

typedef struct
secret { 
int number;
} secret; 

secret* initSecret()
{ 
ERIM_SWITCH_T; 
//manual entry, switch region T 

secret * s = malloc(sizeof(secret)); 

s->number = random(); 
//manual entry, switch region U
ERIM_SWITCH_U; 

return s; 
} 
int compute(secret* s, int m) 
{ 
int ret = 0; 
ERIM_SWITCH_T; 
//manual entry, switch region T 
//f operates in protected context

ret = f(s->number, m); 
//manual entry, switch region U
//end of protected region
ERIM_SWITCH_U; 
return;
}
\end{lstlisting}
\end{subfigure} 
~
\begin{subfigure}[t]{0.45\linewidth}
\vskip 0pt
\centering    
\begin{lstlisting}[language=C,style=CStyle,linewidth=.9\linewidth]
//required Tesseract definitions
mpk_policy(VARIABLE)
mpk_partition(restricted)
...
//annotate protected function prototype
mpk_function_actor(write,restricted) 
int compute(secret* s, int m);

//assign protected member to partition 
typedef struct
mpk_variable_control
(no_access,secret@restricted) 
secret{ int* number; } secret; 

secret* initSecret() { 
//s is automatically inferred to be protected 
secret * s = malloc(sizeof(secret)); 
//explicitly allow write from external function
mpk_access_control(write,restricted)
s->number = random(); 
return s; 
} 
//compute is able to operate on restricted 
int compute(secret* s,int m){
int result;
//do computation no need for manual annotations
return result;
}
\end{lstlisting}
\end{subfigure}
\label{fig:codecomparison}
\end{figure*}
